# Supplementary material for: Toward a Scalable Upper Bound for a CVaR-LQ Problem
Source: arXiv:2103.02136 source file (2022-06-25)
Supplement: Supplementary file 1 [file Appendix.tex]

% \section{Appendix}

% \begin{remark}\label{my23remark}
% Here, we explain how to evaluate the expectation of $W_t W_t^T$ with respect to the probability measure $P_{x,s}^{\pi,\gamma}$ \eqref{myProbMeas}. Note that $W_t$ is not defined on $\Omega$ explicitly but is defined on $\Omega$ \emph{implicitly} through the dynamics $X_{t+1} = AX_t + BU_t + W_t$. For any $(x,s) \in \mathbb{R}^n \times \mathbb{R}$, $\pi \in \Pi$, and $\gamma \in \Gamma$, we have
% \begin{equation}\label{105}\begin{aligned}
%     & E_{x,s}^{\pi,\gamma}(W_t W_t^T) \\
%     & = \textstyle \int_{\mathbb{R}^n} \delta_x(\mathrm{d}x_0) \Big(\int_{\mathbb{R}} \delta_s(\mathrm{d}s_0) \Big(\int_{\mathbb{R}^m}  \pi_0(\mathrm{d}u_0|x_0,s_0)\\
%     & \hphantom{=} \Big( \textstyle \int_{\mathbb{R}_+} \delta_{g(x_0,u_0)}(\mathrm{d}c_0) \Big(\int_{\mathbb{R}^n} \nu_0(\mathrm{d}w_0) \Big(\int_{\mathbb{R}^n} \delta_{f(x_0,u_0,w_0)}(\mathrm{d} x_1)\\
%     %
%     & \hphantom{=} \Big( \textstyle  \int_{\mathbb{R}} \delta_{s_0-c_0}(\mathrm{d}s_1) \Big( \int_{\mathbb{R}^m}  \pi_1(\mathrm{d}u_1|x_1,s_1) \Big( \int_{\mathbb{R}_+} \delta_{g(x_1,u_1)}(\mathrm{d}c_1) \\
%     %
%     & \hphantom{=} \cdots \\
%     %
%     & \hphantom{=} \textstyle\Big( \int_{\mathbb{R}} \delta_{s_{t-1}-c_{t-1}}(\mathrm{d}s_t) \Big(\int_{\mathbb{R}^m} \hspace{-1mm} \pi_t(\mathrm{d}u_t|x_t,s_t) \Big( \int_{\mathbb{R}_+} \hspace{-1mm} \delta_{g(x_t,u_t)}(\mathrm{d}c_t)\\
%     & \hphantom{=}  \textstyle  \Big(\int_{\mathbb{R}^n} \nu_t(\mathrm{d}w_t) \; w_t w_t^T \Big)\Big)\Big)\Big)\cdots\Big)\Big)\Big)\Big)\Big)\Big)\Big)\Big).
% \end{aligned}\end{equation}
% Note that the integrals $\int_{\mathbb{R}^n} \delta_{Ax_t + B u_t + w_t}(\mathrm{d} x_{t+1})$, $\int_{\mathbb{R}} \delta_{s_t-c_t}(\mathrm{d}s_{t+1})$, $\int_{\mathbb{R}^m} \pi_{t+1}(\mathrm{d}u_{t+1}|x_{t+1},s_{t+1})$, etc., equal one, and thus these integrals are not written in \eqref{105}. Moreover,
% \begin{equation*}\begin{aligned}
%   \textstyle \int_{\mathbb{R}_+} \delta_{g(x_t,u_t)}(\mathrm{d}c_t) & = 1\\
%   \textstyle \int_{\mathbb{R}^m} \pi_t(\mathrm{d}u_t|x_t,s_t) & = 1 \\
%     & \vdots\\
%     \textstyle\int_{\mathbb{R}^m}  \pi_0(\mathrm{d}u_0|x_0,s_0) & = 1\\
%     \textstyle\int_{\mathbb{R}} \delta_s(\mathrm{d}s_0)&  = 1\\
%   \textstyle \int_{\mathbb{R}^n} \delta_x(\mathrm{d}x_0) & = 1,
% \end{aligned}\end{equation*}
% where we evaluate the integrals in \eqref{105} in the order specified by the parentheses, and we conclude that
% \begin{equation}
%     E_{x,s}^{\pi,\gamma}(W_t W_t^T) = \textstyle \int_{\mathbb{R}^n} \nu_t(\mathrm{d}w_t) \; w_t w_t^T.
% \end{equation}
% Similar computations, along with $\int_{\mathbb{R}^n} \nu_t(\mathrm{d}w_t) w_t  = 0_{n\times 1}$ for each $t$, are used to find that $E_{x,s}^{\pi,\gamma}(W_t) = 0_{n \times 1}$ and $E_{x,s}^{\pi,\gamma}(W_i W_j^T) = 0_{n \times n}$ for any $i \neq j$.
% \end{remark}
